# Supplementary material for: Convergent Complex Quasi-Newton Proximal Methods for Gradient-Driven Denoisers in Compressed Sensing MRI Reconstruction
Source: arXiv:2505.04820 source file (2025-10-18)
Supplement: Supplementary file 1 [file SM_SOGDenoiser.tex]

\documentclass[journal,twocolumn]{IEEEtran}%onecolumn
\ifCLASSINFOpdf
  % \usepackage[pdftex]{graphicx}
  % declare the path(s) where your graphic files are
  % \graphicspath{{../pdf/}{../jpeg/}}
  % and their extensions so you won't have to specify these with
  % every instance of \includegraphics
  % \DeclareGraphicsExtensions{.pdf,.jpeg,.png}
\else
  % or other class option (dvipsone, dvipdf, if not using dvips). graphicx
  % will default to the driver specified in the system graphics.cfg if no
  % driver is specified.
  % \usepackage[dvips]{graphicx}
  % declare the path(s) where your graphic files are
  % \graphicspath{{../eps/}}
  % and their extensions so you won't have to specify these with
  % every instance of \includegraphics
  % \DeclareGraphicsExtensions{.eps}
\fi
\hyphenation{op-tical net-works semi-conduc-tor}

\usepackage{graphicx}
\input{defs.tex}
\usepackage{color}
\usepackage{cleveref}
\usepackage{silence}
\WarningFilter{latex}{Text page}
\usepackage{soul}
\theoremstyle{plain} % just in case the style had changed

%\swapnumbers % optional, of course
\newtheorem{thm}{Theorem}[section] % the main one
\newcommand{\thistheoremname}{}
\newtheorem{genericthm}[thm]{\thistheoremname}

\newtheorem*{genericthm*}{\thistheoremname}
\newenvironment{namedthm*}[1]
  {\renewcommand{\thistheoremname}{#1}%
   \begin{genericthm*}}
  {\end{genericthm*}}

\usepackage{mathtools, cuted}
\usepackage{relsize}
\usepackage[export]{adjustbox}
\usepackage[dvipsnames]{xcolor}
\usepackage[skins]{tcolorbox}

\definecolor{darkred}{rgb}{0.6,0,0}
\definecolor{darkgreen}{rgb}{0,0.5,0}
\definecolor{darkblue}{rgb}{0,0,0.5}
\definecolor{goldenrod}{rgb}{0.85, 0.65, 0.13}
\definecolor{goldenbrown}{rgb}{0.6, 0.4, 0.08}
\usepackage{tikz,pgfplots}
\pgfplotsset{compat=1.5.1}
\usepgfplotslibrary{groupplots}
%\usepgflibrary{fpu}
%\usepackage{pgfplots}

\usepackage{multicol}

\usepackage{slashbox}
\usepackage{diagbox}
%\usepackage[font=small]{caption} %normalsize % footnotesize

%\usetikzlibrary{intersections,calc,arrows,matrix,spy,math,calc,fit,positioning,decorations, decorations.pathmorphing}
%\tikzset{snake it/.style={decorate, decoration=snake}}
% \pgfplotsset{
%        table/search path={figs/,figs/sim3D},
%    }
%\usetikzlibrary{arrows.meta,shapes.geometric}
%\newcommand{\tikzcircle}[2][red,fill=red]{\tikz[baseline=-0.5ex]\draw[#1,radius=#2] (0,0) circle ;}%
%\DeclareRobustCommand{\tikzarr}[4]{\tikz[baseline=0ex]\draw[-{Latex}] (#1,#2) -- (#3,#4);}

\begin{document}
%
% paper title
% Titles are generally capitalized except for words such as a, an, and, as,
% at, but, by, for, in, nor, of, on, or, the, to and up, which are usually
% not capitalized unless they are the first or last word of the title.
% Linebreaks \\ can be used within to get better formatting as desired.
% Do not put math or special symbols in the title.
\title{Supplementary Material: Convergent Complex Quasi-Newton Proximal Methods for Gradient-Driven Denoisers in Compressed Sensing MRI Reconstruction}
%\title{Convergent Complex Quasi-Newton Proximal Methods
%for Gradient-Driven Denoisers
%\\ in Compressed Sensing MRI Reconstruction}

% Compressed Sensing 
% author names and IEEE memberships
% note positions of commas and nonbreaking spaces ( ~ ) LaTeX will not break
% a structure at a ~ so this keeps an author's name from being broken across
% two lines.
% use \thanks{} to gain access to the first footnote area
% a separate \thanks must be used for each paragraph as LaTeX2e's \thanks
% was not built to handle multiple paragraphs
%

\author{
Tao Hong \IEEEmembership{Member, IEEE}, Zhaoyi Xu, Se Young Chun \IEEEmembership{Member, IEEE}, Luis Hernandez-Garcia, \\
and Jeffrey A. Fessler \IEEEmembership{Fellow, IEEE}

% Zhaoyi Xu, Luis Hernandez-Garcia, and Jeffrey A. Fessler,  \IEEEmembership{Member, IEEE}, \IEEEmembership{Member, IEEE}
% Jeremias Sulam, Se Young Chun  Umberto Villa,  Jason Hu, \IEEEmembership{Member, IEEE}

% \thanks{T. Hong and L. Hernandez-Garcia are with the Department of Radiology, University of Michigan, Ann Arbor, MI 48109, USA (Email: {\{tahong, hernan\}@umich.edu}). TH and LH were partially supported by National Institutes of Health grant R01NS112233.} TH was with the Department of Radiology,
%University of Michigan, Ann Arbor, MI 48109, USA

\thanks{T. Hong is with the Oden Institute for Computational Engineering and Sciences,
University of Texas at Austin, Austin, TX 78712, USA (Email: \texttt{tao.hong@austin.utexas.edu}). TH was with the Department of Radiology, University of Michigan, Ann Arbor, MI 48109, USA. TH was partially supported by NIH grant R01NS112233.
%and R01EB034261.
}
%R01 EB034261
\thanks{Z. Xu is with the Department of Mechanical Engineering,
University of Michigan, Ann Arbor, MI 48109,  USA
(Email: \texttt{zhaoyix@umich.edu}).}

\thanks{S. Chun is with the Department of ECE, INMC \& IPAI, SNU, Seoul, 08826, South Korea
(Email: \texttt{sychun@snu.ac.kr}). SC was partially supported by IITP grant funded by the Korea government (MSIT) [No.RS-2021-II211343, Artificial Intelligence Graduate School Program (Seoul National University)].}
\thanks{L. Hernandez-Garcia is with the Department of Radiology, University of Michigan, Ann Arbor, MI 48109, USA
(Email: \texttt{hernan@umich.edu}). LH was partially supported by NIH grant R01NS112233.}

\thanks{J. Fessler
is with the EECS Department,
University of Michigan, Ann Arbor, MI 48109, USA 
(Email: \texttt{fessler@umich.edu}).
Supported in part by NIH grants
R01EB035618 and R21EB034344.
}

}

% note the % following the last \IEEEmembership and also \thanks - 
% these prevent an unwanted space from occurring between the last author name
% and the end of the author line. i.e., if you had this:
% 
% \author{....lastname \thanks{...} \thanks{...} }
%                     ^------------^------------^----Do not want these spaces!
%
% a space would be appended to the last name and could cause every name on that
% line to be shifted left slightly. This is one of those "LaTeX things". For
% instance, "\mrmbf{A} \mrmbf{B}" will typeset as "A B" not "AB". To get
% "AB" then you have to do: "\mrmbf{A}\mrmbf{B}"
% \thanks is no different in this regard, so shield the last } of each \thanks
% that ends a line with a % and do not let a space in before the next \thanks.
% Spaces after \IEEEmembership other than the last one are OK (and needed) as
% you are supposed to have spaces between the names. For what it is worth,
% this is a minor point as most people would not even notice if the said evil
% space somehow managed to creep in.

% The paper headers
\markboth{}%IEEE Signal Processing Letters, VOL. , NO. , 2019
{Shell \MakeLowercase{\mrmit{et al.}}: Bare Demo of IEEEtran.cls for IEEE Journals}
% The only time the second header will appear is for the odd numbered pages
% after the title page when using the twoside option.
% 
% *** Note that you probably will NOT want to include the author's ***
% *** name in the headers of peer review papers.                   ***
% You can use \ifCLASSOPTIONpeerreview for conditional compilation here if
% you desire.

% If you want to put a publisher's ID mark on the page you can do it like
% this:
%\IEEEpubid{0000--0000/00\$00.00~\copyright~2015 IEEE}
% Remember, if you use this you must call \IEEEpubidadjcol in the second
% column for its text to clear the IEEEpubid mark.

% use for special paper notices
%\IEEEspecialpapernotice{(Invited Paper)}

% make the title area
\maketitle

% As a general rule, do not put math, special symbols or citations
% in the abstract or keywords.
% \begin{abstract}

% \end{abstract}
% Note that keywords are not normally used for peerreview papers.
% \begin{IEEEkeywords}
% Inverse problem, Wavelet based, TV based.
% \end{IEEEkeywords}

% For peer review papers, you can put extra information on the cover
% page as needed:
% \ifCLASSOPTIONpeerreview
% \begin{center} \bfseries EDICS Category: 3-BBND \end{center}
% \fi
%
% For peerreview papers, this IEEEtran command inserts a page break and
% creates the second title. It will be ignored for other modes.
\IEEEpeerreviewmaketitle

\section{Additional Ground Truth Test Images}
In addition to the two brain and knee images presented in the main paper, we also evaluated the performance of our approach on ten additional brain and knee images. \Cref{fig:BrainKneeGT:add} presents the additional test images used in our experiments.

\begin{figure*}%[H]%[t]
    \centering
    \subfigure[2]{\includegraphics[scale=0.5]{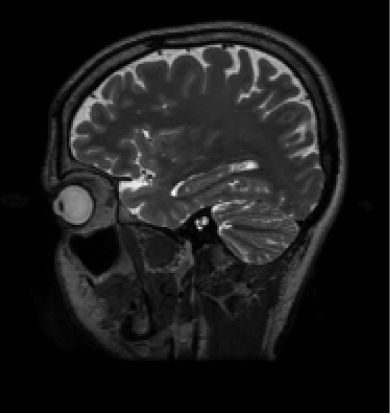}}
    \subfigure[3]{\includegraphics[scale=0.5]{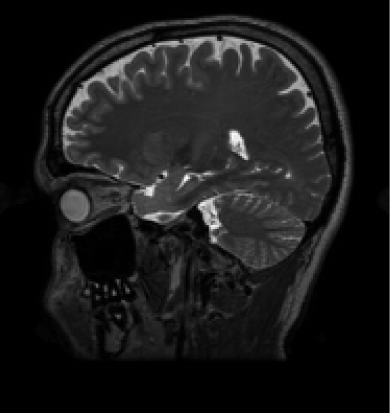}}
    \subfigure[4]{\includegraphics[scale=0.5]{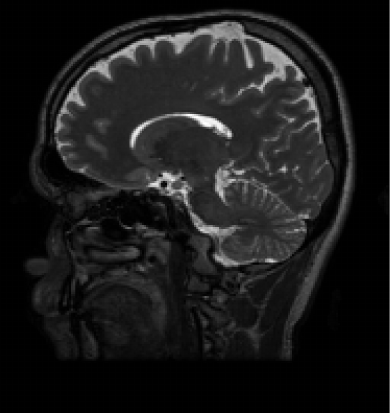}}
    \subfigure[5]{\includegraphics[scale=0.5]{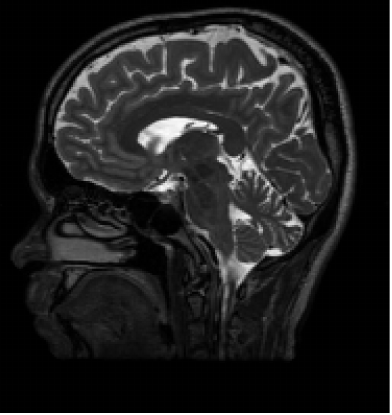}}
     \subfigure[6]{\includegraphics[scale=0.5]{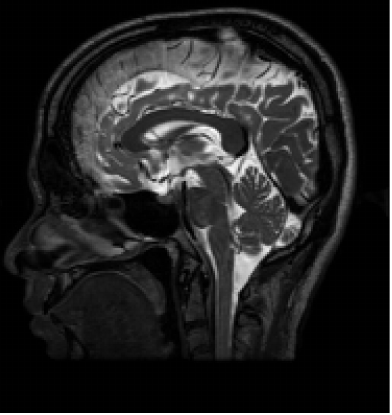}}

    \subfigure[2]{\includegraphics[scale=0.5]{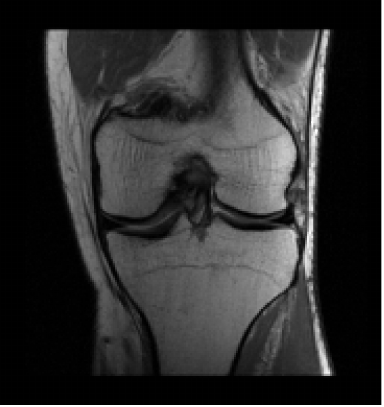}}
    \subfigure[3]{\includegraphics[scale=0.5]{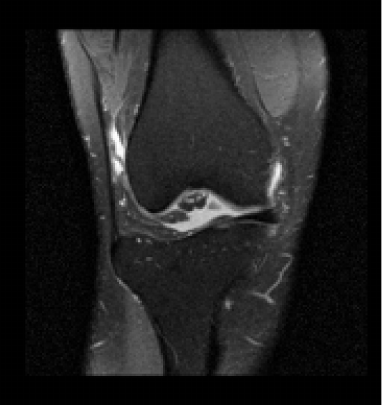}}
    \subfigure[4]{\includegraphics[scale=0.5]{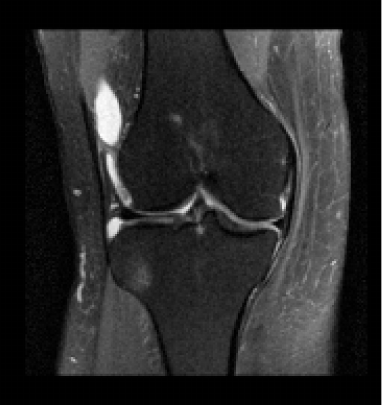}}
    \subfigure[5]{\includegraphics[scale=0.5]{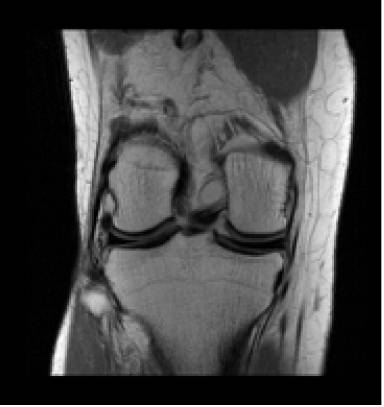}}
    \subfigure[6]{\includegraphics[scale=0.5]{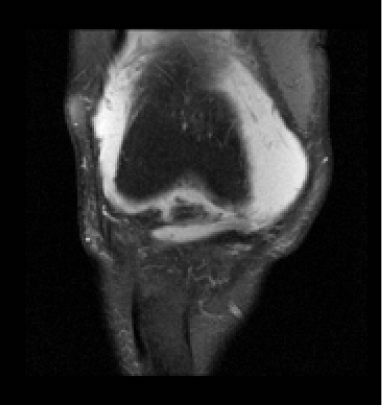}}
    \caption{The magnitude of the five additional brain and knee complex-valued ground-truth images.}
    \label{fig:BrainKneeGT:add}
\end{figure*}

\section{Spiral Acquisition Reconstruction}
This section presents additional experimental results for spiral acquisition. \Cref{fig:SpiralKnee1CostPSNR} shows the cost and PSNR values with respect to the number of iterations and wall time on the knee image. \Cref{fig:SpiralKnee1:visual} displays the reconstructed images and the corresponding error maps for each method at $50$ and $100$th iterations. We observed the same trends as those reported in the main paper. 

Additionally, we ran GD for $500$ iterations on five additional brain images and examined the number of iterations and wall time required for other methods to surpass its performance. \Cref{tab:SpiralBrainOthers} summarizes the results. It is obvious that our method outperformed others in terms of speed. Similar trends were observed for the knee images, as shown in \Cref{tab:SpiralKneeOthers}.

\section{Radial Acquisition Reconstruction}
This section presents additional experimental results for radial acquisition. \Cref{fig:RadialBrain1CostPSNR} shows the cost and PSNR values with respect to the number of iterations and wall time on the brain image. \Cref{fig:RadialBrain1:visual} displays the reconstructed images and the corresponding error maps for each method at $50$ and $100$th iterations. We observed the same trends as those reported in the main paper. 

Additionally, we ran GD for $500$ iterations on five additional knee images and examined the number of iterations and wall time required for other methods to surpass its performance. \Cref{tab:RadialKneeOthers} summarizes the results. It is clear that our method outperformed others in terms of speed. Similar trends were observed for the brain images, as shown in \Cref{tab:RadialBrainOthers}.

\section{Cartesian Acquisition Reconstruction}
We ran GD for $500$ iterations on five additional brain images and examined the number of iterations and wall time required for other methods to surpass its performance. \Cref{tab:CartesianBrainOthers} summarizes the results. It is apparent that our method outperformed others in terms of speed. 

\input{figs_SM/RadialBrainCostRecoIm}

% \bibliographystyle{IEEEtran}
% \bibliography{ResponseTCI/Refs}

\end{document}
